# Supplementary material for: Gamification of Pure Exploration for Linear Bandits
Source: arXiv:2007.00953 source file (2020-07-02)
Supplement: Supplementary file 1 [file oracle_computations.tex]

%!TEX root = ../lin_bandit_explo.tex
\section{Oracle Computations}

\paragraph{Best response.}

Let $x_\mu \in \mathcal A$ be the best action for $\mu$ and $y\in \mathcal A$ different from $x$.
\begin{align*}
\argmin_{\lambda:(y-x_\mu)^\top\lambda \ge 0}\frac{1}{2} \sum_{a \in \mathcal A} w^a (\mu - \lambda)^2_{aa^\top}
&= \mu - \frac{(y-x_\mu)^\top \mu}{\Vert y-x_\mu \Vert^2_{V_w^{-1}}} V_w^{-1}(y - x)
\\
\min_{(y-x_\mu)^\top\lambda \ge 0}\frac{1}{2} \sum_{a \in \mathcal A} w^a (\mu - \lambda)^2_{aa^\top}
&= \frac{1}{2} \frac{((y-x_\mu)^\top \mu)^2}{\Vert y-x_\mu \Vert^2_{V_w^{-1}}}
\end{align*}

\paragraph{Oracle weights.}

The oracle weights are solution of the following problem:
\[
\argmax_{w \in \triangle_K} \min_{y \in \mathcal A} \frac{\Vert y-x_\mu \Vert^2_{\mu \mu^\top}}{\Vert y-x_\mu \Vert^2_{V_w^{-1}}} \quad \text{or equivalently} \quad \argmin_{w \in \triangle_K} \max_{y \in \mathcal A} \frac{\Vert y-x_\mu \Vert^2_{V_w^{-1}}}{\Vert y-x_\mu \Vert^2_{\mu \mu^\top}}
\]
The value of that problem at the optimum is
\[
\max_{w \in \triangle_K} \min_{y \in \mathcal A} \frac{1}{2}\frac{\Vert y-x_\mu \Vert^2_{\mu \mu^\top}}{\Vert y-x_\mu \Vert^2_{V_w^{-1}}}
= \frac{1}{2}\left(\min_{w \in \triangle_K} \max_{y \in \mathcal A} \frac{\Vert y-x_\mu \Vert^2_{V_w^{-1}}}{\Vert y-x_\mu \Vert^2_{\mu \mu^\top}}\right)^{-1}
= \frac{1}{2}H_{LB}^{-1}
\]
where $H_{LB}$ is the complexity defined by~\citet{soare2014linear}.

\paragraph{G-Allocation.}
 
 The G-allocation is defined by~\citet{soare2014linear} as the solution in $w$ of
 \[
\min_{w \in \triangle_K} \max_{x \in \mathcal A} \Vert x \Vert^2_{V_w^{-1}}
 \]

\paragraph{$\mathcal X \mathcal Y$-allocation.}

The $\mathcal X \mathcal Y$-allocation is defined by~\citet{soare2014linear} as the solution in $w$ of
 \[
\min_{w \in \triangle_K} \max_{y,x \in \mathcal A} \Vert y-x \Vert^2_{V_w^{-1}}
 \]

\paragraph{UCB computations.}

\begin{align*}
\left\{\begin{array}{ll}
\sup_\xi \quad &  \frac{1}{2} ((\xi - \lambda)^\top a)^2
\\
\text{s.t.} \quad & \frac{1}{2} \Vert \theta - \xi \Vert^2_V \le \alpha 
\end{array}\right.
&= \max_\pm\frac{1}{2} \left( (\theta - \lambda)^\top a \pm \sqrt{2 \alpha a^\top V^{-1} a} \right)^2
\end{align*}
