# Supplementary material for: Gamification of Pure Exploration for Linear Bandits
Source: arXiv:2007.00953 source file (2020-07-02)
Supplement: Supplementary file 2 [file adaptation_BAI.tex]

%!TEX root = ../lin_bandit_explo.tex
\section{Adaptation to best-arm identification}
In this appendix we explain how to adapt algorithms \algoWCvx and its proof of asymptotic optimality for BAI. The exact same arguments could be used also for \algoW. Indeed in the general case we assume that the set of parameter $\cM$ is bounded which is not the case in BAI and other examples presented in Appendix~\ref{app:examples}. Precisely in the proof of Theorem~\ref{} we only use two times this assumption, first in the definition of the threshold $\beta(t,\delta)$ (see Theorem~\ref{th:confidence_beta}) to handle the bias induced by the regularization. Second in the definition of the upper confidence bounds $U^{i,a}_t$ (see \eqref{eq:def_ucb_br_general}) because AdaHedge requires bounded losses.

One straightforward adaptation is to consider the \emph{bounded} BAI. In this case, the set of parameters is $\cM=\{\theta \in \cR^d:\ |\argmax_{a\in\cA} \langle\theta,a\rangle|=1 \text{ and } \normm{\theta}\leq M\}$, the set of possible answers is $\cI = \cA$ and the correct answer is given by $\istar(\theta)=\astar(\theta)\eqdef \argmax_{a\in\cA} \langle\theta,a\rangle$.
This additional assumption reduces the characteristic time to
\[
\Tstar_b(\theta)^{-1} = \max_{w\in\Sigma_A} \min_{a\neq \astar(\theta)} \inf_{\substack{\langle \lambda,a-\astar(\theta)\rangle>0\\ \normm{\lambda}\leq M}} \normm{\theta -\lambda }_{V_w}^2 \,.
\]
But the best response is less easy to compute, in particular there is no closed formula as for BAI, see Lemma~\ref{lem:lagrange_bounded_BAI}.
\begin{lemma}\label{lem:lagrange_bounded_BAI}
For $\theta, \lambda \in \R^d\,$, $w$ in the interior of the probability simplex $\interior{\Sigma_A}$,
\[
\inf_{\substack{\langle \lambda,a-\astar(\theta)\rangle>0\\ \normm{\lambda}\leq M}} \normm{\theta -\lambda }_{V_w}^2 = \sup_{\gamma\geq 0} \frac{\max\left(\langle \theta, (V_w+\gamma I_d)^{-1} V_w (\astar(\theta)-a)\rangle,0\right)^2 }{2\normm{\astar(\theta)-a}^2_{(V_w+\gamma I_d)^{-1}}}- \frac{\gamma}{2}\left(\normm{\theta}^2-M^2\right)\,,
\]
and if $\gamma$ attains the supremum in the right hand term above then
\[
\lambda = \theta - \frac{\max\left(\langle \theta, (V_w+\gamma I_d)^{-1} V_w (\astar(\theta)-a)\rangle,0\right)}{\normm{\astar(\theta)-a}^2_{(V_w+\gamma I_d)^{-1}}} (V_w+\gamma I_d)^{-1}(a^\star - a)\,.
\]
attains the infimum of left hand term above.
\end{lemma}
\begin{proof}
We set $\astar(\theta) = \astar$. We introduce the Lagrangian
\[
 \inf_{\substack{\langle \lambda,a-\astar \rangle>0\\ \normm{\lambda}\leq M}} \normm{\theta -\lambda }_{V_w}^2 = \sup_{\gamma\geq 0, \alpha\geq 0} \inf_{\substack{\langle \lambda,a-\astar\rangle>0\\ \normm{\lambda}\leq M}} \normm{\theta -\lambda }_{V_w}^2 +\alpha \langle \theta, \astar-a\rangle + \frac{\gamma}{2}\left(\normm{\lambda}^2-M^2 \right)\,.
\]
The infimum above is attained for
\[
\lambda = \theta - \alpha (V_w + \gamma I_d)^{-1}(\astar-a)\,.
\]
Thus the Lagrangian reduces to
\[
\inf_{\substack{\langle \lambda,a-\astar \rangle>0\\ \normm{\lambda}\leq M}} \normm{\theta -\lambda }_{V_w}^2 = \sup_{\gamma\geq 0, \alpha\geq 0}
-\frac{\alpha^2}{2} \normm{\astar-a}^2_{V_w+\gamma I_d} + \alpha \langle \theta, (V_w+\gamma I_d)^{-1}V_w (\astar-a)\rangle +\frac{\gamma}{2}\left(\normm{\theta}^2-M^2 \right)\,.
\]
The supremum in $\alpha$ is reached for
\[
\alpha =\frac{\max\left(\langle \theta, (V_w+\gamma I_d)^{-1} V_w (\astar-a)\rangle,0\right)}{\normm{\astar-a}^2_{(V_w+\gamma I_d)^{-1}}}\,.
\]
Using this particular $\alpha$ in the definition of $\lambda$ and in the Lagrangian allows us to conclude.
\end{proof}

An other possibility is to consider a regularized version of the BAI. Indeed we can remove the need of a bound on $\theta$ for the threshold by using the least square estimator
\[
\ttheta_t = V_{N_t}^{-1} \sum_{s=1}^t Y_s\,,
\]
assuming that we pull all the arms once at the beginning. Thanks to Theorem~\ref{???} we can choose a threshold, independent of $\normm{\theta}$ which is still of order $\beta(\delta,t) = \log(1/\delta) + \text{Poly}\big(\log(t),\log\log(1/\delta)\big)$\,.
